# Supplementary material for: HoloGarment: 360{\deg} Novel View Synthesis of In-the-Wild Garments
Source: arXiv:2509.12187 source file (2025-09-15)
Supplement: Supplementary file 1 [file supp_comparisons.tex]

\begin{figure}[h]
  \centering
  \includegraphics[width=0.9\linewidth]{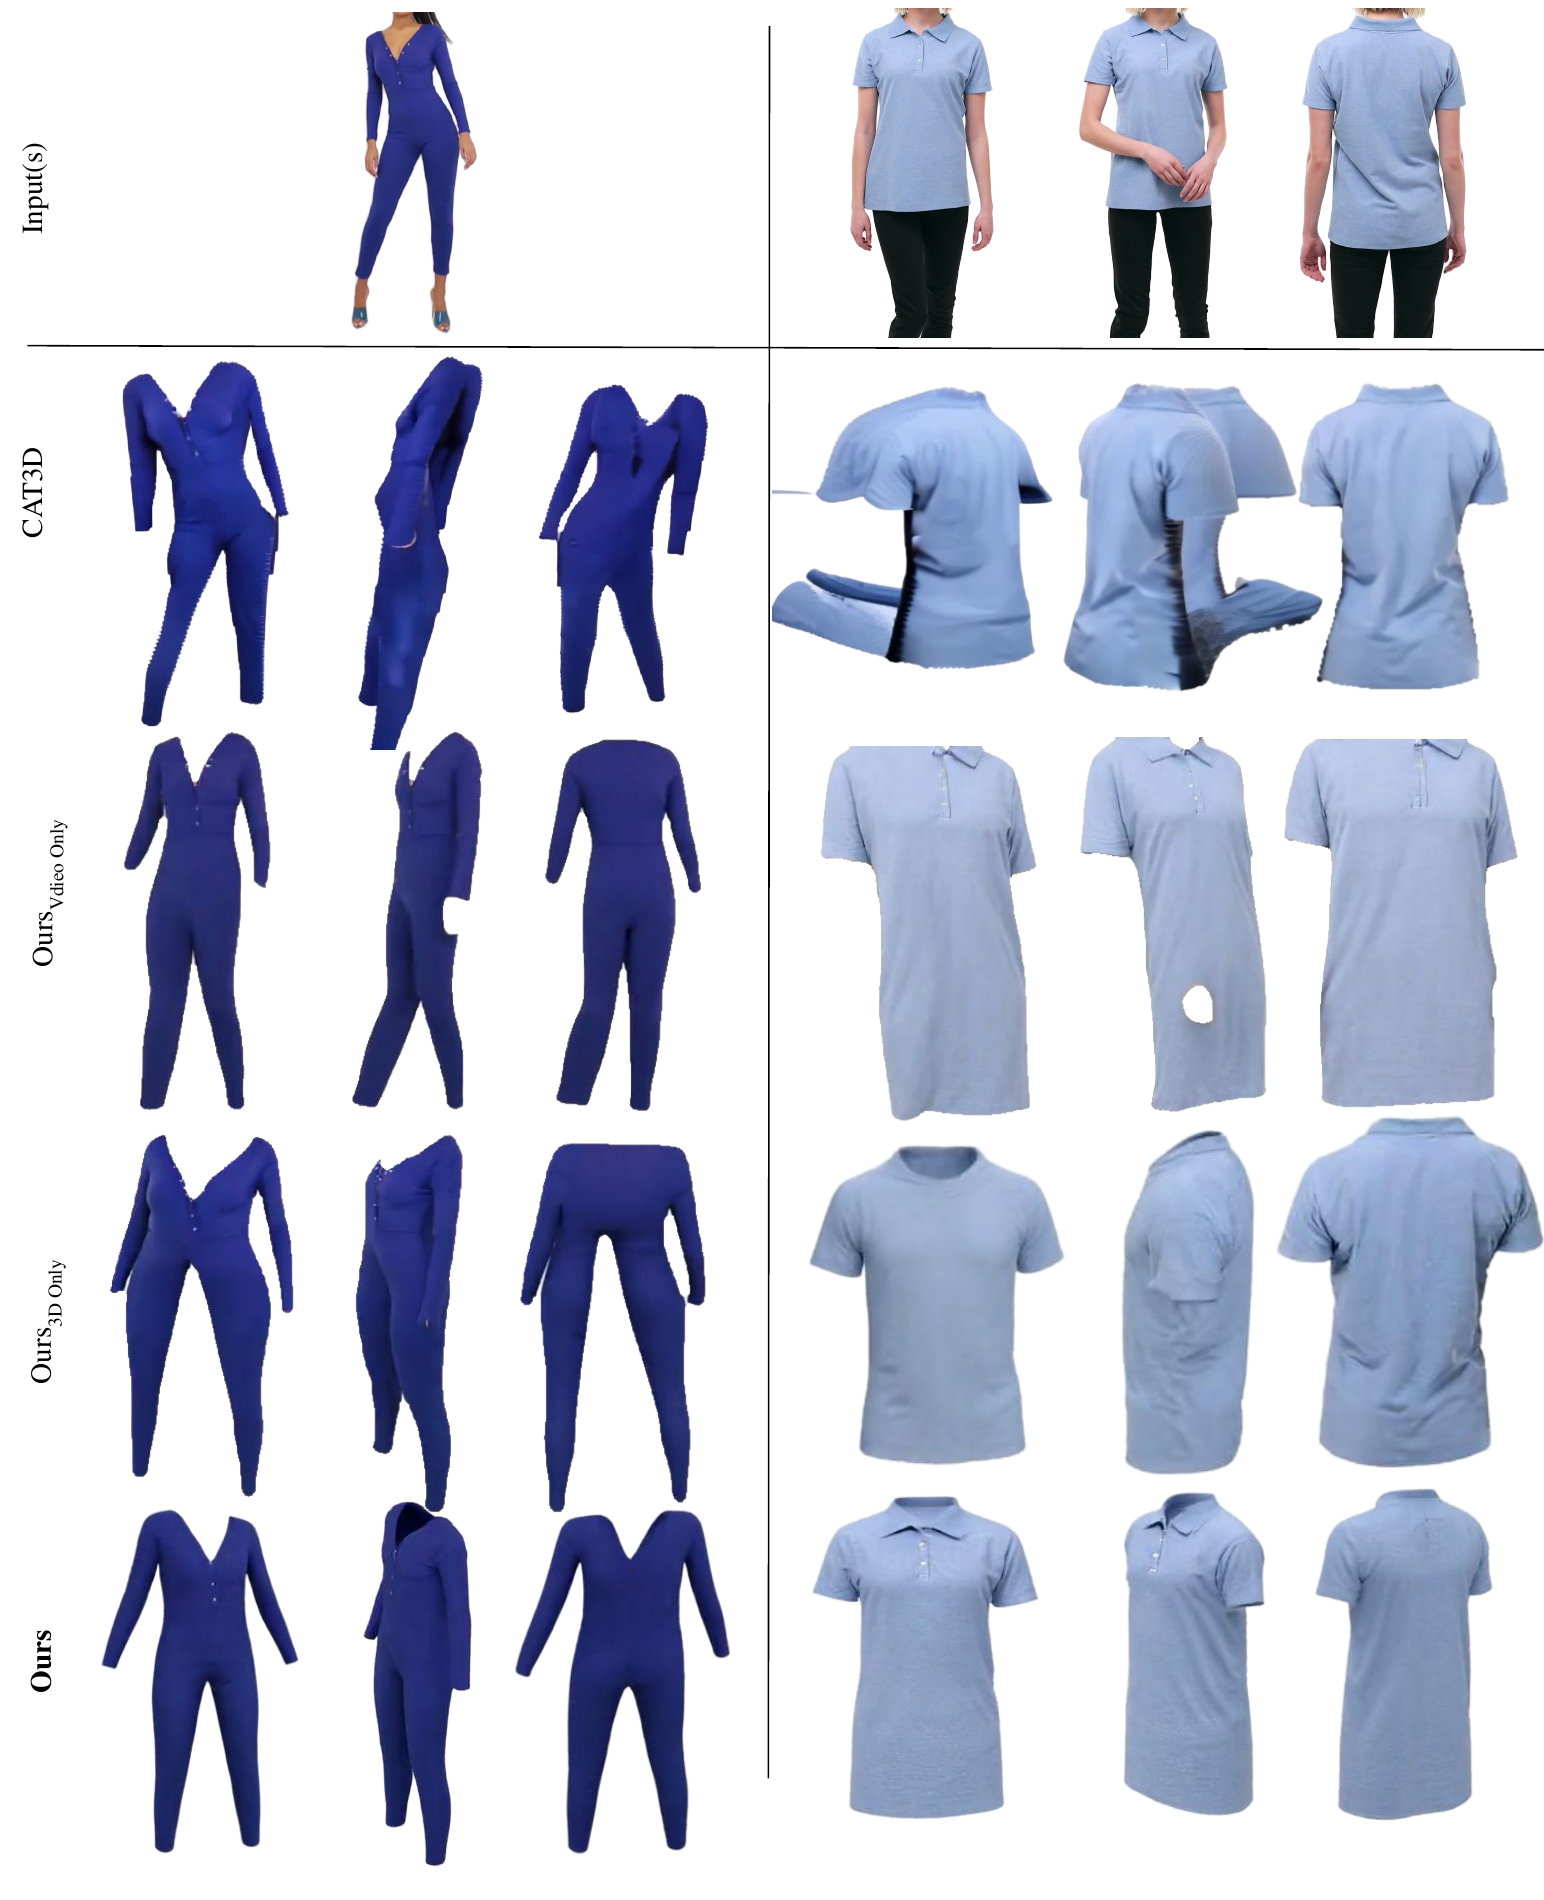}
  \caption{Additional Qualitative Comparisons: We show additional qualitative comparison results for HoloGarment ($\textit{bottom row}$), CAT3D~\citep{cat3d} ($\textit{second row}$), and ablated versions ($\textit{third and fourth rows}$). }
  \label{fig:supp_comparisons}
\end{figure}
